# Supplementary material for: Mitigating Ambiguities in 3D Classification with Gaussian Splatting
Source: arXiv:2503.08352 source file (2025-03-19)
Supplement: Supplementary file 1 [file X_suppl.tex]

\clearpage
\setcounter{page}{1}
\maketitlesupplementary

\section{GS Point Cloud Dataset}
\label{sec:dataset}
\cref{fig:dataset} presents GS point clouds and their corresponding rendering results from our GS Point Cloud Dataset, showcasing real-world examples across various categories.

\begin{figure*}[h]
\centering
\includegraphics[width=\linewidth]{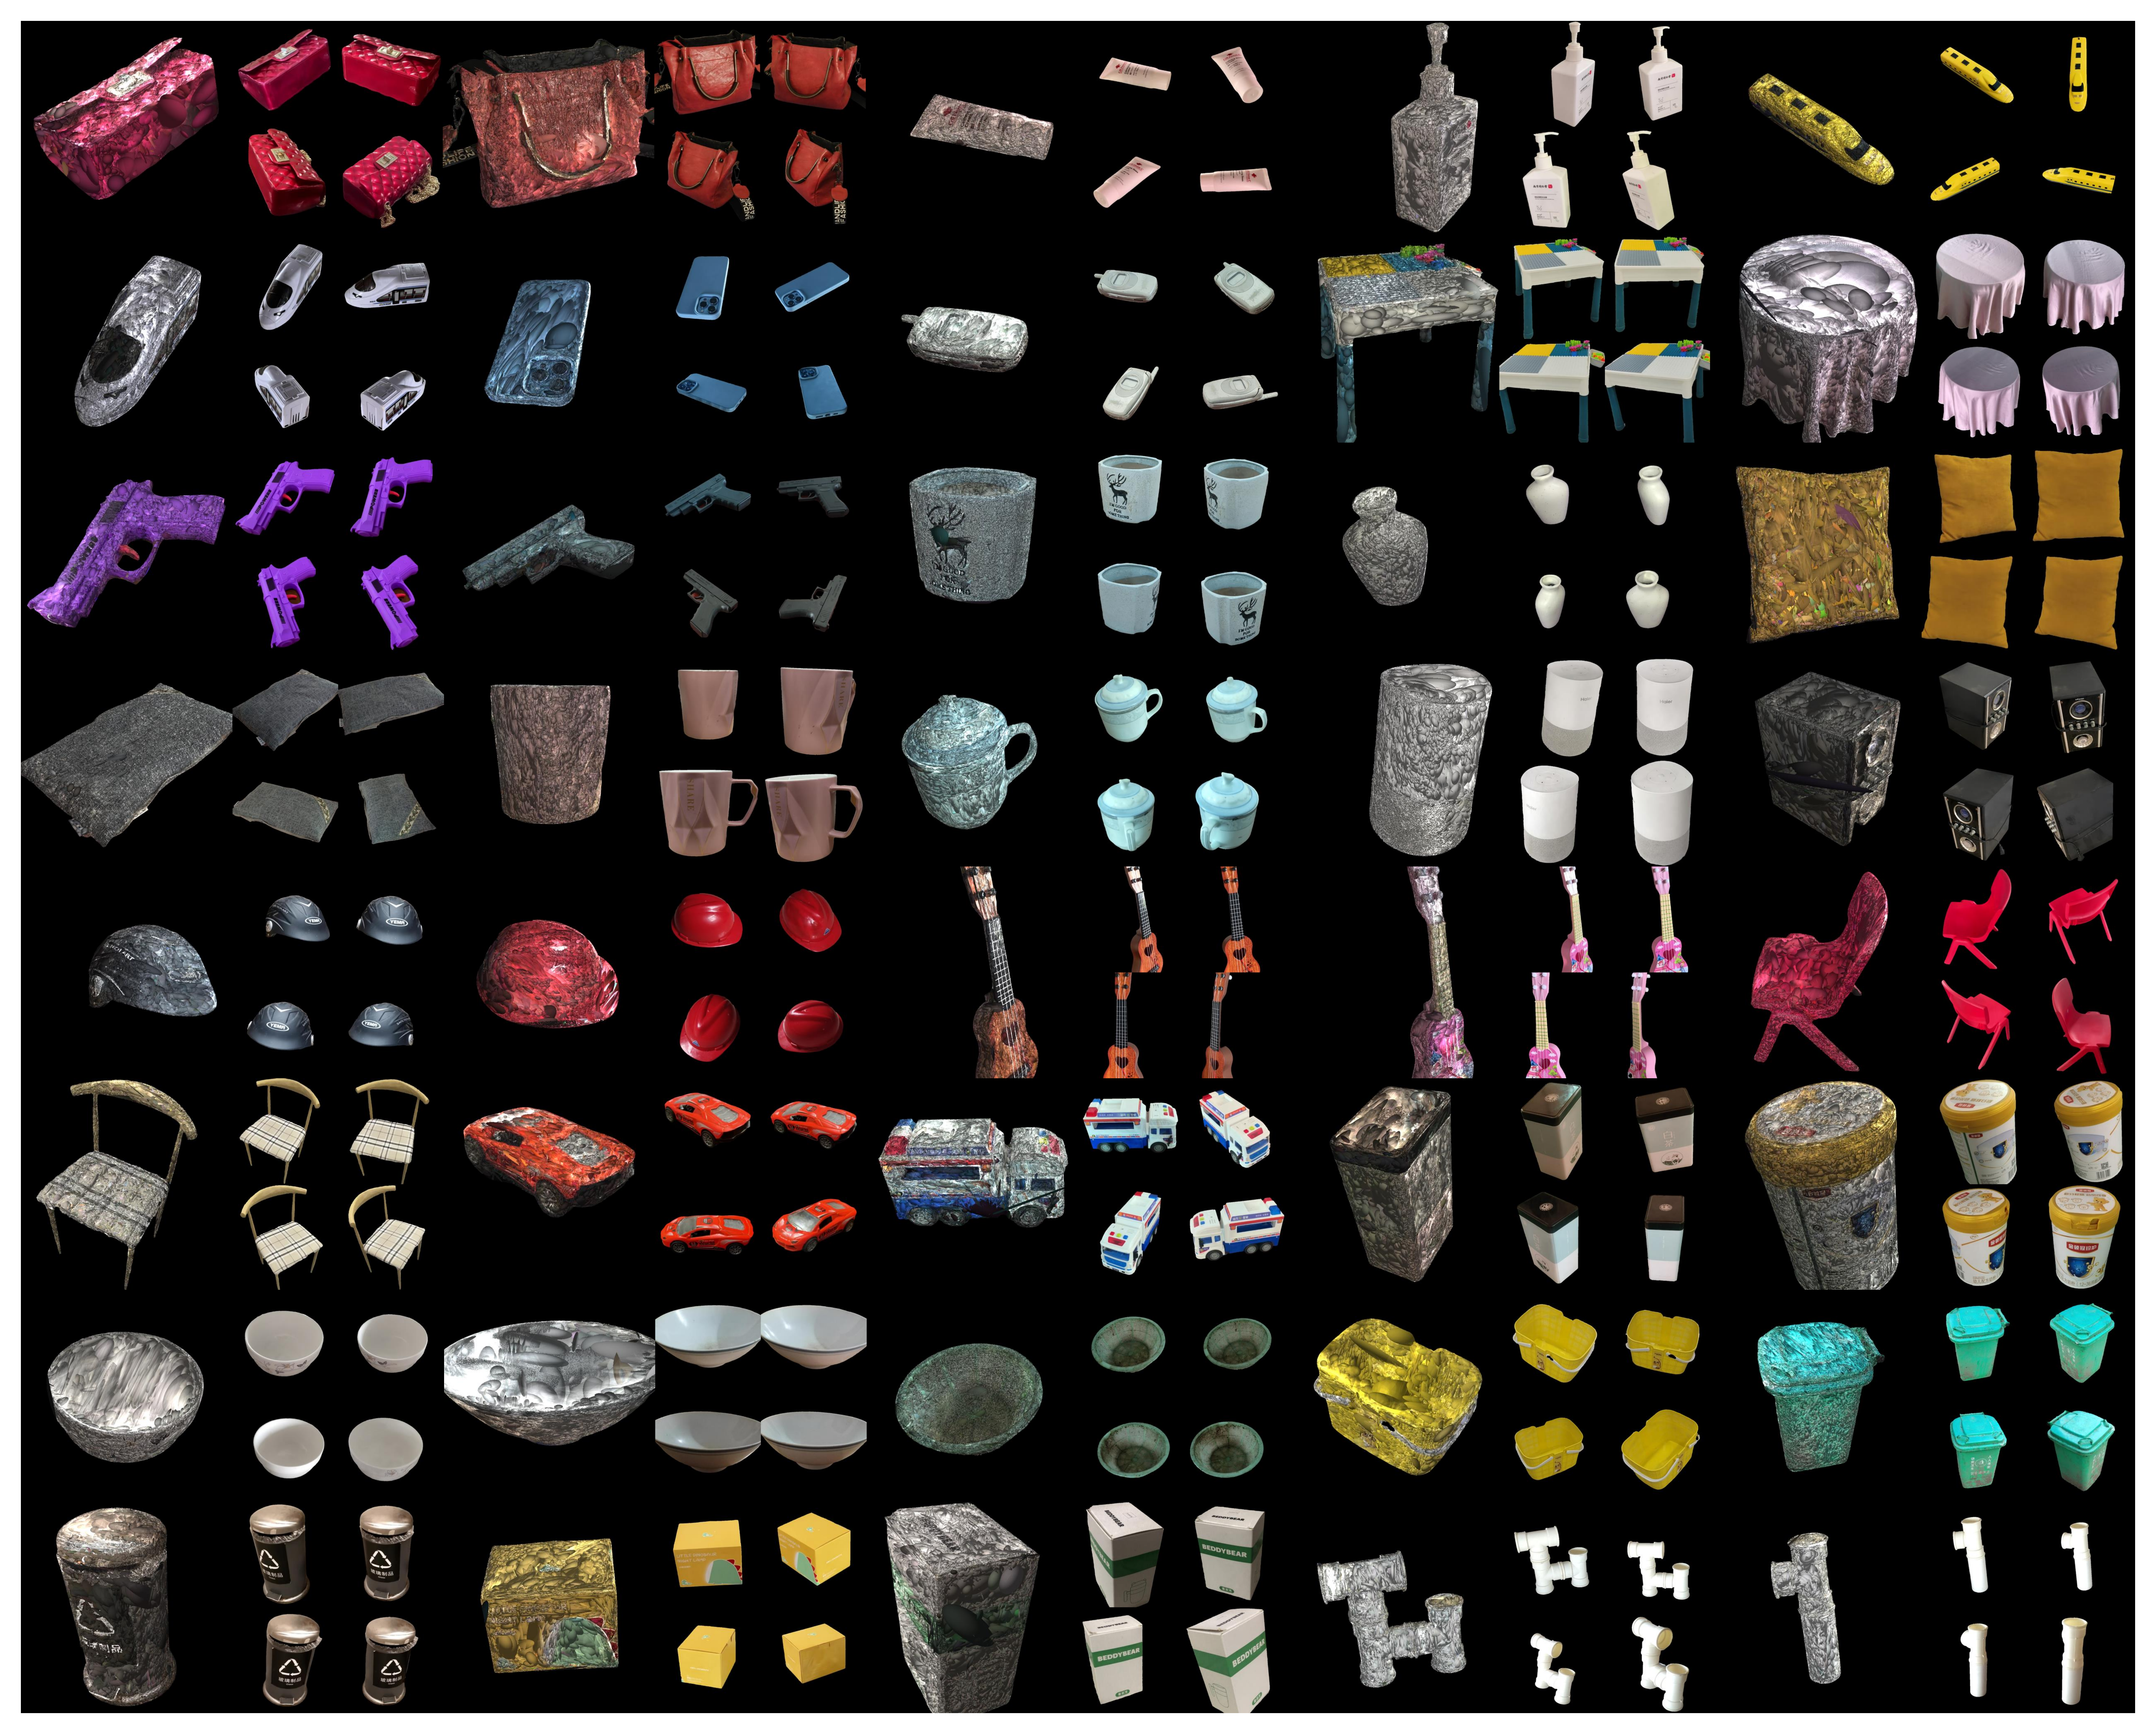} % Reduce the figure size so that it is slightly narrower than the column.
\caption{Visualization of GS point clouds and their corresponding rendering results from our GS Point Cloud Dataset.}
\label{fig:dataset}
\vspace{-0.3cm}
\end{figure*}
% ********************************************************
\clearpage
\section{Features Visualization}
\label{sec:t-SNE}

\cref{fig:pointnet++_tsne,fig:pointnext_tsne,fig:pointmlp_tsne} provide additional t-SNE visualization results for PointNet++~\cite{qi2017pointnet++}, PointNeXt~\cite{qian2022pointnext}, and PointMLP~\cite{ma2022rethinking}.

\begin{figure*}[h]
\centering
\includegraphics[width=\linewidth]{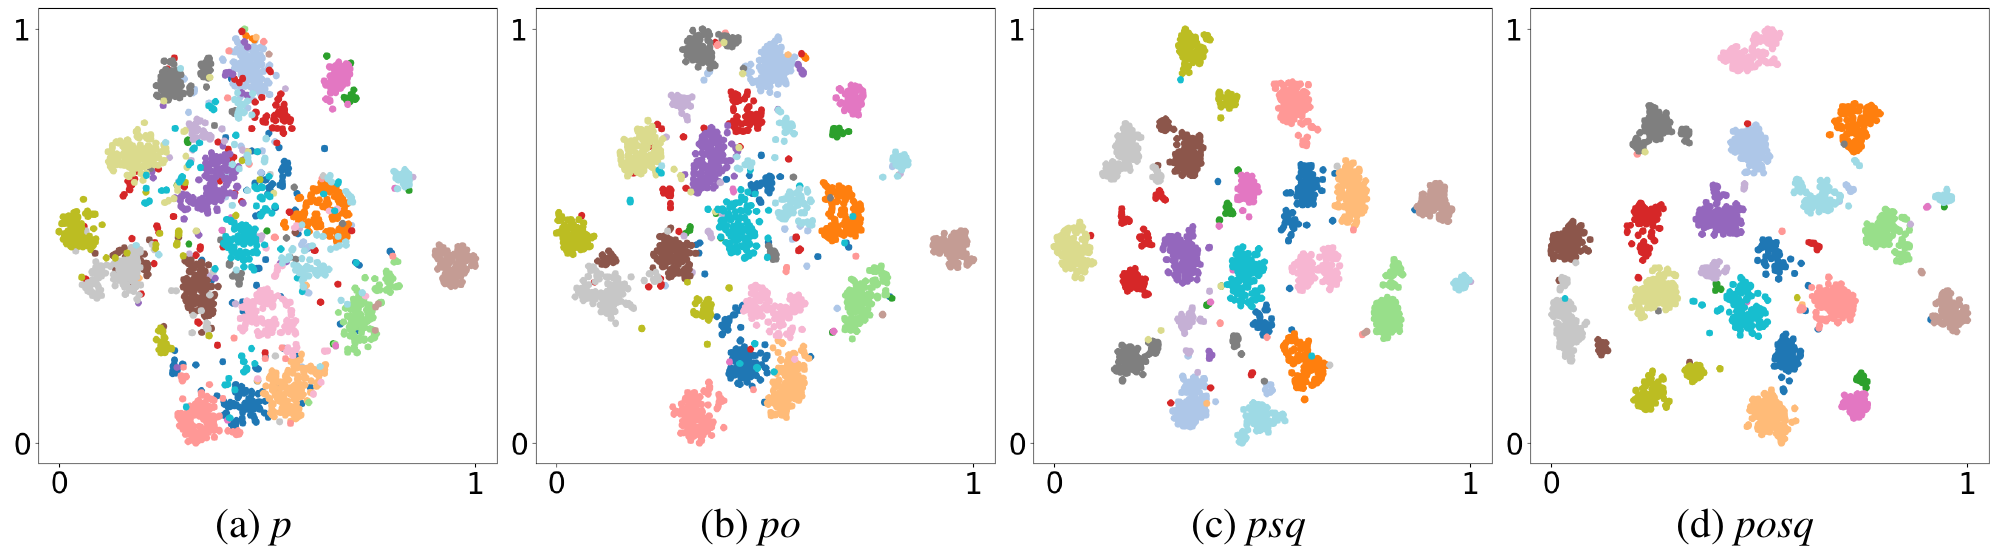} % Reduce the figure size so that it is slightly narrower than the column.
\caption{Visualizations of the global features in PointNet++ with different inputs using t-SNE technique. (a)-(d) are visualized features of network with only position, position+opacity, position+scale+rotation and position+opacity+scale+rotation inputs, respectively.}
\label{fig:pointnet++_tsne}
\vspace{-0.3cm}
\end{figure*}

\begin{figure*}[h]
\centering
\includegraphics[width=\linewidth]{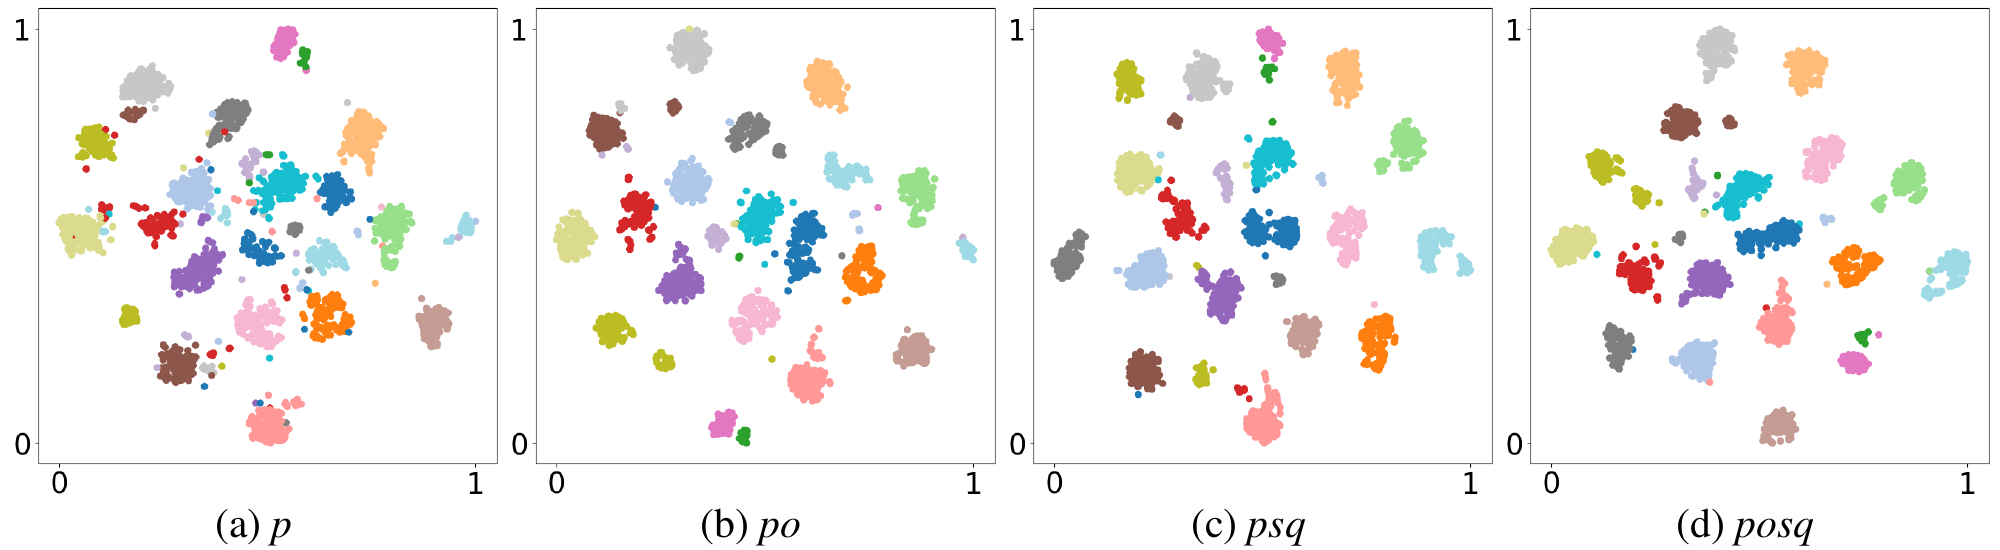} % Reduce the figure size so that it is slightly narrower than the column.
\caption{Visualizations of the global features in PointNeXt with different inputs using t-SNE technique. (a)-(d) are visualized features of network with only position, position+opacity, position+scale+rotation and position+opacity+scale+rotation inputs, respectively.}
\label{fig:pointnext_tsne}
\vspace{-0.3cm}
\end{figure*}

\begin{figure*}[h]
\centering
\includegraphics[width=\linewidth]{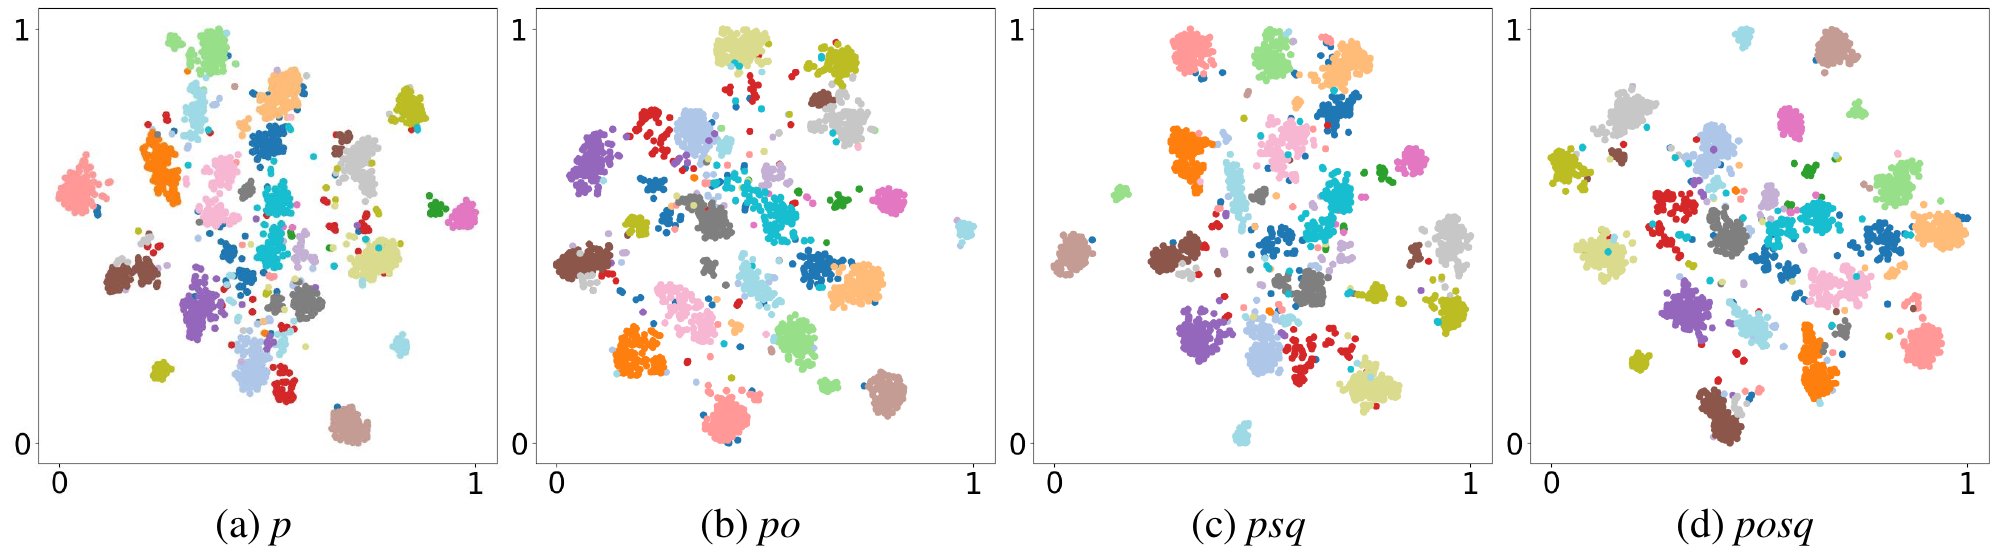} % Reduce the figure size so that it is slightly narrower than the column.
\caption{Visualizations of the global features in PointMLP with different inputs using t-SNE technique. (a)-(d) are visualized features of network with only position, position+opacity, position+scale+rotation and position+opacity+scale+rotation inputs, respectively.}
\label{fig:pointmlp_tsne}
\vspace{-0.3cm}
\end{figure*}
